# Supplementary material for: Towards Distributed 2-Approximation Steiner Minimal Trees in Billion-edge Graphs
Source: arXiv:2205.14503 source file (2022-05-28)
Supplement: Supplementary file 1 [file appendix.tex]

\section{Appendix}
